# Supplementary material for: Explaining the pseudogap through damping and antidamping on the Fermi surface by imaginary spin scattering
Source: arXiv:2107.06529 source file (2023-06-12)
Supplement: Supplementary file 1 [file supplemental.pdf]

# Supplementary information – Explaining the pseudogap through damping and antidamping on the Fermi surface by imaginary spin scattering

Friedrich Krien,[1] Paul Worm,[1] Patrick Chalupa,[1] Alessandro Toschi,[1] and Karsten Held[1]
[1]*Institute for Solid State Physics, TU Wien, 1040 Vienna, Austria*

These notes provide additional information on theoretical and method aspects in Section S.1, and additional results supporting the statements of the main text in Section S.2: In Sec. S.1 A, basics of the dual fermion formalism are recounted. In Sec. S.1 B, we motivate our choice of the parquet approximation. In Sec. S.1 C, key aspects of the parquet solver are explained. In Sec. S.1 D, the fluctuation diagnostic is defined. In Sec. S.1 E we show how the parquet solutions can be converged in the pseudogap regime. In Sec. S.1 D, calculation details are listed. In Sec. S.2 A, additional observables and the doping dependence are presented. In Sec. S.2 B, we demonstrate that in a wide doping and interaction range the spin-fermion vertex has a large imaginary part. Finally, in Sec. S.2 C, we show that the diagrammatic approximation Eq. (4) of the the main text holds for the relevant frequencies. In Sec. S.2 D we compare a model for the pseudogap self-energy to the self-energy obtained from our parquet solver. Finally, in Section S.2 E, we present the analytical continuation of the Green's function and self-energy to real frequencies.

## S.1. SUPPLEMENTARY NOTE 1: METHOD

*Note*: We reserve some freedom in the notation, for example, $\Gamma_{kq}$, $\Gamma(k,q)$, and $\Gamma(\mathbf{k},\nu,\mathbf{q},\omega)$ are all equivalent.

### A. Dual formalism and definitions

We employ the method introduced in Ref. [1], which is based on the dual fermion formalism [2], one of several diagrammatic extensions [3–7] of the dynamical mean-field theory (DMFT, [8]). We reiterate here only the definitions needed in relation with the main text. In DMFT one solves the effective Anderson impurity model (AIM),

$$S_{\mathrm{AIM}} = -\sum_{\nu\sigma} c^*_{\nu\sigma}(\imath\nu + \mu - h_\nu)c_{\nu\sigma} + U\sum_{\omega} n_{\uparrow\omega}n_{\downarrow\omega}. \tag{S.1}$$

Here $c^*, c$ are Grassmann variables, $\mu$ the chemical potential, and $\nu$, $\omega$ are the fermionic and bosonic Matsubara frequencies, respectively. Here and in the following, summations over $\nu,\omega$ imply multiplication with the temperature $T=\beta^{-1}$, summations over momenta imply division by the number of lattice sites $N$. The hybridization function $h_\nu$ is fixed according to the prescription $\sum_{\mathbf{k}} G^{\mathrm{DMFT}}_k = g_\nu$, where $G^{\mathrm{DMFT}}$ is the Green's function in DMFT approximation and $g$ is the local Green's function of the AIM. We keep $h_\nu \equiv h^{\mathrm{DMFT}}_\nu$ of DMFT also in our parquet dual fermion calculations.

Our approach requires several higher correlation functions of the AIM:

$$f^\alpha(\nu,\nu',\omega) = \frac{-\frac{1}{2}\sum_{\sigma_i} s^\alpha_{\sigma_1'\sigma_1} s^\alpha_{\sigma_2'\sigma_2}\langle c_{\nu\sigma_1}c^*_{\nu+\omega,\sigma_1'}c_{\nu'+\omega,\sigma_2}c^*_{\nu'\sigma_2'}\rangle - \beta g_\nu g_{\nu+\omega}\delta_{\nu\nu'} + 2\beta g_\nu g_{\nu'}\delta_\omega\delta_{\alpha,\mathrm{ch}}}{g_\nu g_{\nu+\omega} g_{\nu'} g_{\nu'+\omega}}, \tag{S.2}$$

$$\chi^\alpha(\omega) = \langle\rho^\alpha_{-\omega}\rho^\alpha_\omega\rangle - \beta\langle n\rangle\langle n\rangle\delta_\omega\delta_{\alpha,\mathrm{ch}}, \qquad w^\alpha(\omega) = U^\alpha - \frac{1}{2}U^\alpha\chi^\alpha(\omega)U^\alpha, \tag{S.3}$$

$$\Gamma^\alpha_{\mathrm{loc}}(\nu,\omega) = \frac{\frac{1}{2}\sum_{\sigma\sigma'} s^\alpha_{\sigma'\sigma}\langle c_{\nu\sigma}c^*_{\nu+\omega,\sigma'}\rho^\alpha_\omega\rangle + \beta g_\nu\langle n\rangle\delta_\omega\delta_{\alpha,\mathrm{ch}}}{g_\nu g_{\nu+\omega} w^\alpha(\omega)/U^\alpha}. \tag{S.4}$$

The label $\alpha = \mathrm{ch},\mathrm{sp}$ denotes charge or spin flavor, $\rho^{\mathrm{ch}} = n_\uparrow + n_\downarrow = n$ and $\rho^{\mathrm{sp}} = n_\uparrow - n_\downarrow$ the charge and spin density, $U^{\mathrm{ch}} = U$ and $U^{\mathrm{sp}} = -U$ the bare Hubbard interaction for the respective channel. We refer to the various correlation functions as vertex ($f$), susceptibility ($\chi$), screened interaction ($w$), and boson-fermion vertex ($\Gamma_{\mathrm{loc}}$). We focus on its spin part, i.e., the spin-fermion vertex and the corresponding screened interaction; we denote them for simplicity as

$$\Gamma^{\mathrm{sp}}_{\mathrm{loc}} \equiv \Gamma_{\mathrm{loc}}, \quad w^{\mathrm{sp}} \equiv w. \tag{S.5}$$

In practice we use a continuous-time quantum Monte Carlo solver [9] with improved estimators [10] for calculating the particle-hole correlation functions defined above. Our method also requires singlet particle-particle correlation functions [1], which are measured instead using the worm-sampling [11] of w2dynamics [12].

In the dual formalism the Hubbard model is mapped to the action

$$S[d^*,d] = -\sum_{k\sigma}(\tilde{G}^0_k)^{-1}d^*_{k\sigma}d_{k\sigma} + \frac{1}{4}\sum_{kk'q}\sum_{\sigma_i} f^{\sigma_1\sigma_2\sigma_3\sigma_4}_{\nu\nu'\omega} d^*_{k\sigma_1}d^*_{k'+q,\sigma_2}d_{k'\sigma_3}d_{k+q,\sigma_4}, \tag{S.6}$$

Grassmann numbers $d^*, d$ represent the dual fermions, $\tilde{G}^0 = G^{\mathrm{DMFT}} - g$ is the nonlocal DMFT Green's function. Higher than quartic interactions between dual fermions are neglected, as usual done with few exceptions[13, 14]. The dual self-energy is given as,

$$\tilde{\Sigma}_k = \sum_{k'}\tilde{G}_{k'}f^{\mathrm{ch}}_{\nu'\nu,\omega=0} - \frac{1}{4}\sum_{k'q}\tilde{G}_{k+q}\left[F^{\mathrm{ch}}_{kk'q}\tilde{X}^0_{k'q}f^{\mathrm{ch}}_{\nu'\nu\omega} + 3F^{\mathrm{sp}}_{kk'q}\tilde{X}^0_{k'q}f^{\mathrm{sp}}_{\nu'\nu\omega}\right], \tag{S.7}$$

where $\tilde{X}^0_{kq} = \tilde{G}_k\tilde{G}_{k+q}$ denotes a bubble of dual Green's functions $\tilde{G} = [(\tilde{G}^0)^{-1} - \tilde{\Sigma}]^{-1}$ and $F$ is the full vertex of the dual fermions. Both $F$ and $\tilde{G}$ still need to be calculated self-consistently as explained in the next Section.

### B. Choice of approximation

The dual formalism corresponds only to the mapping of the problem of the Hubbard model to the action (S.6), with the purpose of reaching the strong-coupling regime [15, 16] and improving the convergence of diagrams with the

frequency cutoff [17]. The question which diagrams are taken into account for the full vertex $F$ in Eq. (S.7) should be kept separate, in particular, no choice of diagrams corresponds to 'the dual fermion approach/approximation'. Sets of diagrams for the dual vertex $F$ discussed in the literature are the second-order approximation [18, 19], the ladder approximation [7, 13], the parquet approximation [1, 20], and stochastic sampling [21, 22], in ascending order of 'completeness'. Also contributions of higher-order vertices to the dual self-energy have been discussed [14] (which we do not consider here because it undercuts the computational efficiency). The question which diagrams are taken into account is one of physical setting, computational feasibility, convergence, and the need to avoid bias.

In the context of the doped Hubbard model and the pseudogap one often encounters the notion of 'competing orders'. To be unbiased in this respect one needs to include the feedback between the different channels without making an a priori choice, i.e., take the parquet diagrams into account. At the outset of this work we expected that competing or exotic orders may play a role in the formation of the pseudogap, but the explanation for the pseudogap given in the main text does not require competing orders. It may therefore seem that the ladder approximation [3, 13] is sufficient, which takes the feedback of magnetic fluctuations on the self-energy into account. In fact, the ladder approximation does capture key aspects of the physics described in the main text (see Fig. S.4 below). However, it would not be convincing to base the arguments in the main text only on the ladder approximation for the following reasons:

*First*, of central importance for our explanation of the pseudogap is the spin-fermion vertex $\Gamma$. In the ladder approximation this quantity is given as [17]

$$\Gamma(\nu,q) = \Gamma_{\rm loc}(\nu,\omega) + \sum_{\nu'}[f^{\rm sp}(\nu,\nu',\omega) - \Gamma_{\rm loc}(\nu,\omega)w(\omega)\Gamma_{\rm loc}(\nu',\omega)]\tilde{X}^0(\nu',q)\Gamma(\nu',q), \tag{S.8}$$

where $\tilde{X}^0(\nu',q) = \sum_{\mathbf{k}} \tilde{X}^0_{kq}$. Since in the ladder approximation vertex corrections are local, $\Gamma$ does not depend on the fermionic momentum $\mathbf{k}$. Physically this means that the coupling to paramagnons is the same for all fermions, which is an atavism that can be traced back to the DMFT approximation. However, in the pseudogap regime an extreme nodal/antinodal dichotomy develops and we have to expect that fermions near the nodes are coupled differently to paramagnons than those near the antinodes. This is indeed the case, as in the pseudogap regime the Adler principle applies to the Fermi arcs, but not to momenta where the pseudogap opens (see main text). We discuss the ladder approximation for $\Gamma$ again further below in Sec. S.2 B.

*Second*, the presence of strong local correlations introduces a large eigenvalue in the charge channel (see also Fig. S.2). This is plausible due to the Ward identity which implies that

$$\lim_{\omega\to 0}\lim_{\mathbf{q}\to 0}\Gamma^{\rm ch/sp}(\mathbf{k},\nu=0,\mathbf{q},\omega) \propto \left(1 - \left.\frac{d\Sigma(\mathbf{k},\nu)}{d\nu}\right|_{\nu=0}\right), \tag{S.9}$$

where $\nu,\omega$ are real frequencies in this equation. For a Fermi liquid the right-hand-side corresponds to the inverse quasi-particle weight $Z_{\mathbf{k}}^{-1}$ (this underlines again that the $\mathbf{k}$-dependence of $\Gamma$ is important when $Z_{\mathbf{k}}$ is strongly anisotropic). The vertex is thus enhanced in the strongly correlated regime where $Z$ is small. On Matsubara frequencies this is connected to a large eigenvalue of the Bethe-Salpeter equation for *finite* frequencies $\omega$ (because $\mathbf{q}$ must go to zero first), in particular for $\omega_1 = 2\pi T$ (see Fig. S.2).

This effect is already present in DMFT, leading to a divergence of the boson-fermion vertex at the zero-temperature Mott transition [23]. Interestingly, Eq. (S.9) is valid both in the charge and in the spin channel but in practical calculations using Matsubara frequencies the corresponding eigenvalue is much larger in the charge channel [23], presumably because the Mott gap is a charge gap. A large eigenvalue at finite frequency has been observed also in fRG studies [24, 25]. Strong local correlations ('Mottness') are a sufficient, but not a necessary condition for this eigenvalue to be large. (It should not be confused with the eigenvalue associated to $\alpha = \text{ch}, \mathbf{q} = 0, \omega = 0$, which corresponds to the phase separation instability, even though phase separation and the Mott transition often go hand in hand [23, 26].)

However, in DMFT and also in the ladder dual fermion approximation the large eigenvalue has no feedback on other channels; including this feedback requires at least the parquet diagrams. Although the Ward identity is violated by the parquet approximation [27] we do find the corresponding large eigenvalue, which for strong coupling is in fact the leading instability for all considered dopings (see panel (b) of Fig. S.3). Hence, to avoid a potential source of bias we allow the mutual renormalization of the different channels via the parquet diagrams.

*Third*, even in absence of competition, a strong fluctuation can interact with itself in the sense of an effective $\phi^4$-theory [28–30]. It was shown by Bickers and Scalapino [31] that this 'self-renormalization' is included in the parquet diagrams; in terms of the $1/N$ expansion the parquet is comparable to the so-called self-consistent screening approximation [32]. In the Bethe-Salpeter equation this feedback corresponds to the renormalization of the irreducible vertex. However, in the ladder approximation the latter is fixed and local, cf. Eq. (S.8), and hence the self-renormalization of bosonic fluctuations is neglected in the ladder approximation [33]. It is indeed the case that the accuracy of the

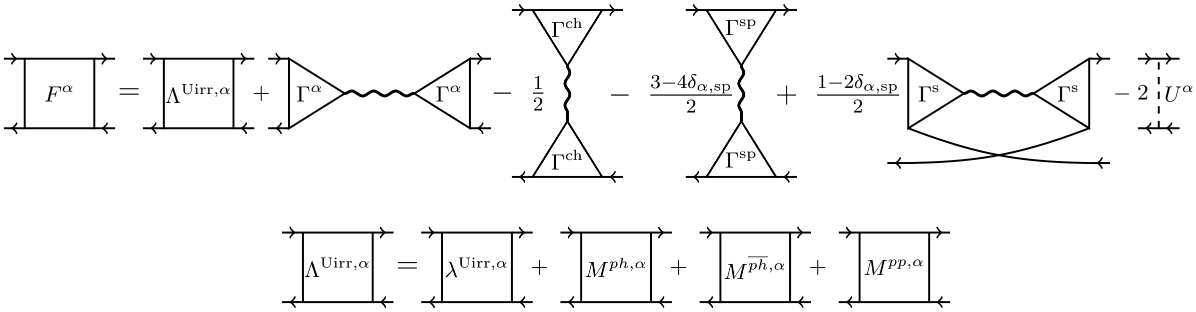

Supplementary Figure S.1: Double decomposition of the vertex function according to Ref. [1]. Top: Single-boson exchange decomposition of the full vertex [36]. The momentum dependence of the fermion-boson vertices is fully retained. Bottom: Parquet equation for the multi-boson exchange. The momentum dependence of the four-point vertices is parameterized using the truncated unity [37].

ladder approximation worsens at the onset of the pseudogap regime [34], where spin fluctuations are strong, while it is improved by the parquet diagrams [35].

### C. Parquet solver

We explain aspects of the parquet solver for dual fermions presented in Ref. [1] relevant for the main text.

For a long time, since the introduction of the parquet approach, the full solution of the parquet equations on a large lattice was considered to be computationally unfeasible. Applications to impurity models and small clusters were pioneered in Refs. [38–42], see Ref. [43] for a review. The computational bottleneck is the memory required to store the various vertex functions [44]. Very recently, based on concepts used in the fRG [45–47], progress was made to compress the information encoded in the parquet vertices, which depend on three momenta and three frequencies. The expansion and truncation of vertices in a form-factor basis allows to treat much larger lattice sizes [37, 48], for example, a vertex quantity $\Phi$ is transformed as,

$$\Phi(\mathbf{k},\nu,\mathbf{k}',\nu',\mathbf{q},\omega)\to\Phi(\ell,\nu,\ell',\nu',\mathbf{q},\omega), \tag{S.10}$$

where $\ell,\ell'$ denote form-factor indices (corresponding in our case to the form factors of the square lattice). The change of basis is exact, but only a small number of form factors is kept (truncated unity). This corresponds to cutting off the respective momentum argument in real space (cf. Fig. 7 of Ref. [37]). That is, discarding form factors with index $\ell>\ell_{\max}$ implies to cut off $\Phi(\mathbf{r},\nu,\mathbf{r}',\nu',\mathbf{q},\omega)$ with respect to $\mathbf{r},\mathbf{r}'$, the Fourier conjugate variables of $\mathbf{k},\mathbf{k}'$, respectively. The truncated-unity approximation is therefore suitable when the vertex quantity $\Phi$ is *short-ranged* in real space.

However, in the pseudogap regime spin fluctuations are longer-ranged, in particular at weak coupling [34, 35], but also at strong coupling a number of nearest neighbor shells should be taken into account. To remedy this, the parquet diagrams were regrouped in Refs. [1, 49] in terms of single- and multi-boson exchange [36], as shown in Fig. S.1. The regrouping of diagrams is exact and therefore has no effect on the parquet approximation itself. But the convergence with the number of form factors can be improved drastically, as we explain in the following.

The single-boson exchange (SBE) diagrams carry the bare momentum argument of the fluctuation and hence should not be truncated in real space. For example, for spin fluctuations the SBE diagram reads,

$$\Delta(\mathbf{k},\nu,\mathbf{k}',\nu',\mathbf{q},\omega)=\Gamma(\mathbf{k},\nu,\mathbf{q},\omega)\,W(\mathbf{q},\omega)\,\Gamma(\mathbf{k}',\nu',\mathbf{q},\omega), \tag{S.11}$$

where $W$ is the screened interaction. In the method of Ref. [1] the full momentum dependence of $\Gamma$ and $W$ is retained. The diagrams $\Delta$ of SBE type are constructed in the horizontal [cf. Eq. (S.11)] and vertical particle-hole channels, and in the particle-particle channel, see top of Fig. S.1 and Ref. [36].

On the other hand, the residual vertex $\Lambda^{\rm Uirr}$ in Fig. S.1 corresponds to multi-boson exchange (notice that $\lambda^{\rm Uirr}$ is a local residual vertex [36] and vertices $M$ represent multi-boson exchange in the horizontal and vertical particle-hole channels and in the particle-particle channel [1]). This vertex is much more short-ranged compared to the full vertex $F$ because the momentum argument of spin fluctuations appears only under integrals. This makes the multi-boson exchange amenable for the truncated-unity approximation [1, 49]. As a result, the form-factor expansion for $\Lambda^{\rm Uirr}$ converges quickly, even in the presence of very long-ranged spin-density wave fluctuations. In principle, the

convergence with the form factors could worsen if $\Lambda^{\mathrm{Uirr}}$ develops a strong momentum dependence. In the pseudogap regime at weak coupling [35] this is not observed.

For the strong-coupling regime the effect of higher form factors will be investigated elsewhere. In the main text we show the self-energy computed with only one form factor. This allows us to reach small dopings efficiently (cf. Sec. S.1 E); tests for larger dopings (not shown) did not reveal a major effect if further form factors are included. The reason for this is that the particle-particle channel is not yet important; if $d$-wave superconducting fluctuations develop alongside antiferromagnetic spin fluctuations further form factors are required to capture their competition. Nevertheless, even in this case a single form factor may still describe qualitatively the correct physics [48].

As Eq. (S.11) shows, the spin-fermion vertex is not only a passive output that we can compute using the parquet vertices but a central quantity which is stored and updated over the iterations. It is obtained from the full vertex as,

$$\Gamma(k,q) = \Gamma_{\mathrm{loc}}(\nu,\omega) + \sum_{k'}[F^{\mathrm{sp}}(k,k',q) - \Delta(k,k',q)]\tilde{X}^0(k',q)\Gamma_{\mathrm{loc}}(\nu',\omega). \tag{S.12}$$

In contrast to the ladder approximation in Eq. (S.8), $\Gamma$ inherits the complete momentum dependence from the full vertex function $F$. We can hence capture the nodal/antinodal dichotomy of $\Gamma$ in the pseudogap regime. The dual screened interaction $W$ is obtained from $\Gamma$ through

$$W(q) = \frac{w(\omega)}{1 - w(\omega)\Pi(q)}, \quad \Pi(q) = \sum_k \Gamma_{\mathrm{loc}}(\nu,\omega)\tilde{X}^0(k,q)\Gamma(k,q), \tag{S.13}$$

where $\Pi$ is the dual polarization.

### D. Fluctuation diagnostic

In the main text we are interested in the contribution of spin fluctuations to the (dual) self-energy. This idea has been coined a 'fluctuation diagnostic' [50–54] which we adopt here, but with two modifications [35, 55].

*First,* we are not interested in a fluctuation diagnostic of local correlations. They instead are our baseline against which we compare the contribution of nonlocal correlations. Fortunately, this separation of local and nonlocal correlations is already intrinsic to the dual formalism where the approximation for the self-energy of the real fermions is given as,

$$\Sigma(k) = \Sigma^{\mathrm{DMFT}}(\nu) + \frac{\tilde{\Sigma}(k)}{1 + g(\nu)\tilde{\Sigma}(k)}. \tag{S.14}$$

Here, $\Sigma^{\mathrm{DMFT}}$ is the local self-energy of the self-consistent AIM (S.1) of DMFT. Notice that while local and nonlocal correlations are separated, there remains some ambiguity in the choice of the hybridization function $h_\nu$ of the AIM. While this may lead to quantitative differences and shifts between $\Sigma^{\mathrm{DMFT}}$ and $\sum_{\mathbf{k}} \tilde{\Sigma}(k)/[1+g(\nu)\tilde{\Sigma}(k)]$, the mechanism that opens the pseudogap is intrinsically nonlocal and does not depend on this choice. In the literature good results have been obtained using $h^{\mathrm{DMFT}}$ or by fixing $h$ using the prescription $\tilde{G}_{\mathrm{loc}} = 0$ [18, 22, 35, 56].

*Second,* the original fluctuation diagnostic is based on the Fierz ambiguity and one adopts one of three equivalent reference frames (charge, spin, or particle-particle [50, 53]). In the dual formalism the Fierz ambiguity is however reduced due to the fact that the bare interaction $f^{\mathrm{ch/sp}}$ has a flavor. Instead, we make use of the decomposition into SBE diagrams intrinsic to our method (cf. Fig. S.1). We obtain the contribution of single spin fluctuations to the self-energy according to Ref. [35],

$$\tilde{\Sigma}_{\mathrm{sp}}(k) = -\frac{3}{2}\sum_{k'q}\tilde{G}(k+q)\Delta(k,k',q)\tilde{X}^0(k',q)f^{\mathrm{sp}}(\nu',\nu,\omega). \tag{S.15}$$

In the main text we are interested in the contribution of nonlocal spin fluctuations to the imaginary part $\Sigma''$ of the lattice self-energy (S.14). The denominator $1 + g(\nu)\tilde{\Sigma}(k)$ in Eq. (S.14) is complex but its real part is leading and we can hence focus our attention on $\tilde{\Sigma}''_{\mathrm{sp}}$. Using (S.11) we write Eq. (S.15) as

$$\tilde{\Sigma}_{\mathrm{sp}}(k) = -\frac{3}{2}\sum_q \tilde{G}(k+q)\Gamma(k,q)W(q)\tilde{\Gamma}(\nu,q), \tag{S.16}$$

where we defined the vertex quantity

$$\tilde{\Gamma}(\nu,q)=\sum_{k'}\Gamma(k',q)\tilde{X}^0(k',q)f^{\mathrm{sp}}(\nu',\nu,\omega). \tag{S.17}$$

In a perturbation theory for real fermions with the bare vertex $U$ this diagram would correspond to the polarization times $U^{\mathrm{sp}}$ and using the Dyson equation for $W$ Eq. (S.16) would assume a $GW\Gamma$-like form. However, in the dual formalism the bare vertex $f$ depends on three frequencies and Eq. (S.17) is not the polarization diagram [cf. Eq. (S.13)]. We therefore have to include the above-defined $\tilde{\Gamma}$ into the discussion which is similar to $\Gamma$ but does not depend on $\mathbf{k}$. We take the imaginary part of Eq. (S.16) and separate by real and imaginary part of $\tilde{G}$,

$$\tilde{\Sigma}''_{\mathrm{sp}}(k)=-\frac{3}{2}\sum_q\left[\tilde{G}'_{k+q}(\Gamma'_{kq}\tilde{\Gamma}''_{\nu q}+\Gamma''_{kq}\tilde{\Gamma}'_{\nu q})+\tilde{G}''_{k+q}(\Gamma'_{kq}\tilde{\Gamma}'_{\nu q}-\Gamma''_{kq}\tilde{\Gamma}''_{\nu q})\right]W_q. \tag{S.18}$$

This is the dual analog to the model self-energy $GW\Gamma$ used in the main text. The key feature that they share is that the real part $\tilde{G}'$ of the dual Green's function contributes to $\tilde{\Sigma}''_{\mathrm{sp}}$ only via the imaginary part of a vertex. A difference is that in Eq. S.18 both $\Gamma$ or $\tilde{\Gamma}$ enter. However, the latter is anyhow defined in terms of the former via Eq. S.17. Hence, in the dual fermion theory we also have a kind of $GW\Gamma$ form as in the spin-fermion ansatz [Eq. (2) main text], just with a few complications: (i) the denominator in Eq. (S.14) is a complex number, (ii) we had to introduce a second vertex $\tilde{\Gamma}$, (iii) the imaginary part $\tilde{G}''$ of the dual Green's function can be positive, (iv) the imaginary parts $\Gamma'',\tilde{\Gamma}''$ couple not only to $\tilde{G}'$ but (in their combination) also to $\tilde{G}''$. Despite these complications our numerical results presented in the main text show full consistency with the qualitative predictions based on the model self-energy $GW\Gamma$ for real fermions.

### E. Convergence in the pseudogap regime

Technical details and implementation notes for our method are provided in Ref. [1]. We add here a note to explain how calculations are converged in the pseudogap regime using Anderson/Pulay mixing.

In the parquet iterations the following large vector of quantities is updated self-consistently:

$$\mathbf{x}_i=(\tilde{\Sigma}_i,\Pi_i^\alpha,\Gamma_i^\alpha,\Lambda_i^{\mathrm{Uirr},\alpha}). \tag{S.19}$$

As an initial guess for $\mathbf{x}_0$, in most cases a converged ladder dual fermion calculation is used where the ladder self-energy $\tilde{\Sigma}_0$ in Eq. (S.8) yields $\Gamma_0$ and then $\Pi_0$ via Eq. (S.13); $\Lambda_0^{\mathrm{Uirr}}=0$ is a reasonable initial guess. As discussed in relation with Eq. (S.8), $\Gamma_0(\nu,q)$ does not depend on $\mathbf{k}$ in the ladder approximation, but $\Gamma_i$ acquires this dependence already after the first parquet iteration.

In Eq. (S.19) $\tilde{\Sigma}(k),\Pi(q)$, and $\Gamma(k,q)$ carry the full momentum and frequency dependence, but not $\Lambda^{\mathrm{Uirr}}$ which represents a set of vertex functions (the multi-boson exchange, cf. Fig. S.1). These vertices are parameterized in terms of the truncated form-factor basis [cf. right-hand-side of Eq. (S.10)], which drastically reduces the required memory. In our calculations outside of the pseudogap regime linear mixing converges fast, which is defined as,

$$\mathbf{x}_{i+1}=(1-\xi)\mathbf{x}_i+\xi\mathbf{g}[\mathbf{x}_i],\quad(0<\xi\leq 1), \tag{S.20}$$

where $\mathbf{g}$ is the result of the parquet iteration. However, at smaller dopings, as soon as the quasiparticle weight is suppressed near the antinodes, convergence deteriorates and linear mixing fails.

Slow convergence often has a physical origin, for example, critical slowing down of the iterative cycle of DMFT sets in near the Mott transition when a solution turns from stable to unstable as a function of a control parameter (interaction, temperature, doping, ...). The free energy landscape around the minimum is then very flat. For DMFT it was shown that stability of the iterative cycle is determined by the *dual* Bethe-Salpeter kernel $\sum_{\nu'}f^{\mathrm{ch}}_{\nu\nu',\omega=0}\tilde{X}^0_{\nu',q=0}$ [16], which highlights the dual fermion approach [2] as a natural extension of diagrammatic perturbation theory to the strong-coupling regime, and serves as a further justification of our numerical method.

To improve the convergence of the parquet solver we employ Anderson/Pulay mixing which has been used previously to accelerate the iterative cycle of DMFT [57, 58] and its diagrammatic extensions [59]. In the improved mixing scheme one defines a fixed-point function,

$$\mathbf{f}[\mathbf{x}_i]=\mathbf{g}[\mathbf{x}_i]-\mathbf{x}_i\equiv\mathbf{f}_i, \tag{S.21}$$

and the solution $\mathbf{x}^*$ hence satisfies $\mathbf{f}[\mathbf{x}^*]=0$. Convergence of an iterative scheme is determined by the eigenvalues of the Jacobian $\mathcal{J}=\frac{\delta\mathbf{f}}{\delta\mathbf{x}}\big|_{\mathbf{x}^*}$. Convergence of linear mixing deteriorates if an eigenvalue approaches unity. An improved mixing

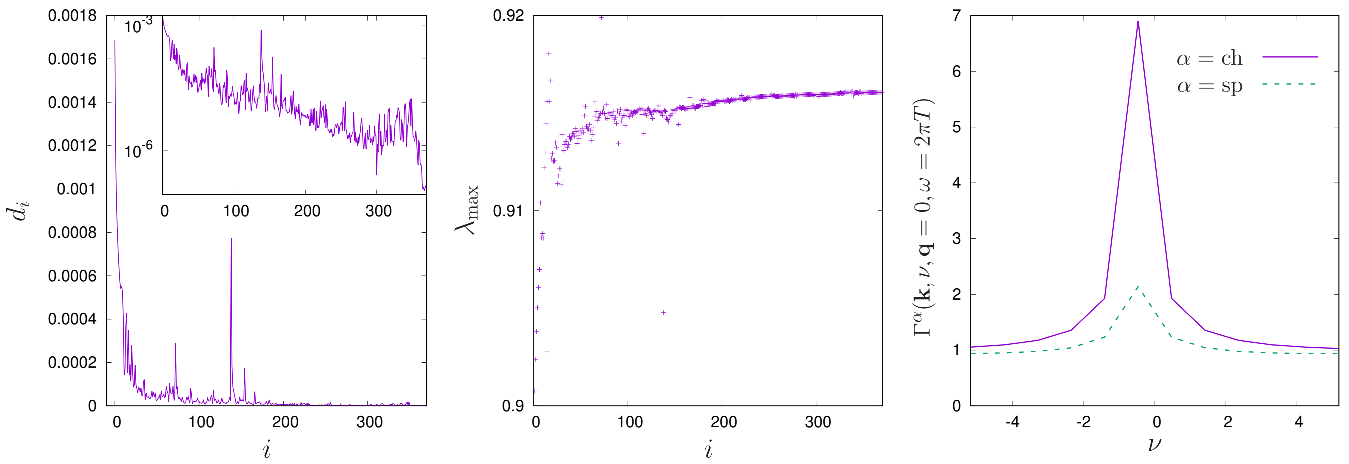


Supplementary Figure S.2: Convergence of the parquet solver in the pseudogap regime ($T/t = 0.15, \delta = 0.01$), updates are computed using the 5 previous iterations as input. Left: Decay of the distance function of the dual self-energy over the iterations, the inset shows a logarithmic scale. The calculation was stopped after 370 iterations at an accuracy $d < 10^{-7}$. Center: Leading eigenvalue in the charge channel for $\mathbf{q} = 0, \omega = 2\pi T$. Right: Enhancement of the charge vertex at the antinode. Here the enhancement is due to 'Mottness', i.e., strong local correlations suppress the quasiparticle weight $Z$ [cf. Eq. (S.9)].

scheme approximates $\mathcal{J}$, based on $\mathbf{f}_i, \mathbf{f}_{i-1}, \ldots$ evaluated at previously traversed points $\mathbf{x}_i, \mathbf{x}_{i-1}, \ldots$, and constructs an update $\mathbf{x}_{i+1}$ taking into account the slope of $\mathbf{f}$. Extrapolating from a sequence of $n+1$ parquet iterations $\mathbf{x}_{i-n}, \ldots, \mathbf{x}_i$, the updated vector is given through the Anderson/Pulay mixing as (cf., e.g., Ref. [60]),

$$\mathbf{x}_{i+1} = \mathbf{x}_i + \hat{C}_i \mathbf{f}_i, \tag{S.22}$$

$$\hat{C}_i = \xi \hat{1} - (\mathbf{R}_i + \xi \mathbf{F}_i)([\mathbf{F}_i]^T \mathbf{F}_i)^{-1} [\mathbf{F}_i]^T, \tag{S.23}$$

$$\mathbf{R}_i = (\mathbf{x}_{i-n+1} - \mathbf{x}_{i-n}, \mathbf{x}_{i-n+2} - \mathbf{x}_{i-n+1}, \ldots, \mathbf{x}_i - \mathbf{x}_{i-1}), \tag{S.24}$$

$$\mathbf{F}_i = (\mathbf{f}_{i-n+1} - \mathbf{f}_{i-n}, \mathbf{f}_{i-n+2} - \mathbf{f}_{i-n+1}, \ldots, \mathbf{f}_i - \mathbf{f}_{i-1}). \tag{S.25}$$

Unfortunately, due to the full momentum and frequency dependence of $\Gamma(k, q)$ it is not feasible to store this quantity for many iterations. Therefore, we apply linear mixing in the subspace of $\Gamma$, where the respective matrix elements of $\hat{C}_i$ are set to $\xi \hat{1}$. Similarly, we apply the improved mixing only to the smallest frequencies of $\Lambda^{\mathrm{Uirr}}$ and linear mixing to higher frequencies.

Using the improved mixing scheme we are able to converge also in the pseudogap regime. The left panel of Fig. S.2 shows the distance $d_i = |\tilde{\Sigma}_i - \tilde{\Sigma}_{i-1}|$ (normalized by the length of the array) as a function of $i$ for temperature $T/t = 0.15$ and doping $\delta = 0.01$, the most extreme parameters we accessed so far with the described optimizations. Since we have to use linear mixing for $\Gamma$, the improved mixing scheme does not unfold its full power and $d_i$ shows an erratic, weakly exponential decay. Even for well converged solutions we observe sporadically a strong increase of $d_i$, followed by a return to the convergent track.

Overall convergence of the iterative scheme is tightly connected to convergence of the leading eigenvalues [40] of the ladder equations that are discussed in more detail in Ref. [1]. In the strongly correlated regime the leading eigenvalue is in the charge channel, connected to the momentum and energy $q = (\mathbf{q} = 0, \omega = 2\pi T)$, as discussed below Eq. (S.9). We find that this eigenvalue is the origin of the convergence problems in the pseudogap regime at strong coupling. In contrast, in the pseudogap regime at weak coupling [35] this eigenvalue is small, which shows that strong correlations have a destabilizing effect on diagrammatic perturbation theory. The center panel of Fig. S.2 shows the large eigenvalue as a function of the iterations.

At the level of the vertex the large eigenvalue leads to an enhancement of $\Gamma^{\mathrm{ch}}(\mathbf{k}, \nu, \mathbf{q} = 0, \omega = 2\pi T)$, shown in the right panel of Fig. S.2 for $\mathbf{k}$ corresponding to the antinode (but $\mathbf{k}$-dependence of the feature is weak). The spin-fermion vertex $\Gamma^{\mathrm{sp}}$ shows a much smaller enhancement, a disparity also observed in Ref. [23]. The enhancement of the charge vertex and its relation to electron-phonon coupling, phase separation, superconductivity, and charge density waves has been discussed by many authors, see, for example, Refs. [61, 62]. In agreement with Ref. [61] we observe the enhancement only for $|\mathbf{q}| \ll \omega$, where screening is ineffective. Notice that instability of $\Gamma$ is rather the exception than the rule, for example, in the case of strong spin fluctuations $\Gamma^{\mathrm{sp}}$ is even suppressed near $\mathbf{Q}$ (see main text).

In contrast to Ref. [40] we do not encounter convergence problems connected to a violation of the crossing symmetry. This may be a benefit of our bosonized parquet approach, which explicitly preserves the crossing symmetry at the level of the SBE diagrams [cf. Fig. S.1] (the truncated-unity approximation violates the crossing symmetry of $\Lambda^{\rm Uirr}$).

### F. Calculation details

Our parquet calculations were performed on a lattice of size $N = 16\times 16$, as a good compromise between resolution and computational feasibility. The self-energy $\Sigma_\nu^{\rm DMFT}$ of the self-consistent AIM (S.1) of DMFT was evaluated at $N_\nu^{(1)} = 64$ positive Matsubara frequencies. The four-point vertex $f_{\nu\nu'\omega}$ was evaluated at $N_\omega = 14$ bosonic frequencies $\omega_m \geq 0$ and $N_\nu^{(2)} = 14$ fermionic frequencies $\nu_n$ with index $-7 \leq n \leq 6$. The three-point vertices $\Gamma_{\rm loc}(\nu,\omega)$ are evaluated in the same window. The vertices at negative bosonic frequencies $\omega < 0$ can be obtained from the positive frequencies, $f(\nu,\nu',\omega) = f^*(-\nu',-\nu,-\omega)$ and $\Gamma_{\rm loc}(\nu,\omega) = \Gamma^*_{\rm loc}(-\nu,-\omega)$, and hence for the chosen $N_\nu^{(2)}$ and $N_\omega$ the window for bosonic frequencies is twice as large as for fermionic ones. This reduces the cutoff error for fermionic observables, whereas a cutoff error is visible in bosonic observables near $\omega \approx N_\nu^{(2)}/2$. If instead our focus was to evaluate bosonic correlation functions the window for fermionic frequencies should be twice larger than for bosonic ones. While these cutoffs may seem small, our method presented in Ref. [1] is heavily optimized in this respect. Purely local quantities are measured directly by the impurity solver [9, 10], avoiding for example summation over local charge correlation functions whose features are shifted to high energies in the strongly correlated regime [63]. Furthermore, on top of the fast decay of the dual Green's function $\tilde{G} \propto 1/\nu^2$, the bosonization of the parquet equations also leads to the decay of the vertices so that, for example, a Bethe-Salpeter kernel of the form $\tilde{X}^0_{kq} S_{kk'q}$ decays as $\propto 1/\nu^5$ [1, 17].

## S.2. SUPPLEMENTARY NOTE 2: FURTHER SUPPORTING RESULTS

### A. Additional parquet dual fermion observables

To put the results shown in the main text into a broader context we report here several more observables. We first note, however, that diagrammatic approximations based on the dual fermion formalism, including stochastic summation of diagrams, are not fully consistent internally, see Refs. [18, 22] for discussions. This puts some uncertainty on the actual doping level $\delta$, which we obtain from summation over the lattice Green's function $\sum_k G_k$. Further, since the dual formalism heavily relies on directly measured impurity correlation functions [cf. Eqs. (S.2)-(S.4)], the choice of the hybridization function $h_\nu$ becomes important. The best quantitative agreement with numerically exact results has so far been achieved using the prescription $\tilde{G}_{\rm loc} = 0$ [22, 35]. Here we use however the DMFT hybridization $h^{\rm DMFT}$ which yields good results in combination with stochastic sampling [22] and our parquet approach in turn shows good agreement with stochastic sampling where it can be converged in the perturbation order [1]. We emphasize that our goal here is to investigate the strongly coupled Hubbard model for cuprates *qualitatively*; benchmarks against numerically exact methods in this or a similar regime will be presented elsewhere.

Fig. S.3 shows various quantities for our hole-doping scan at $T/t = 0.15$. Panel (a) shows $\Delta\Sigma(\mathbf{k}) = \Sigma(\mathbf{k},\pi T) - \Sigma(\mathbf{k},3\pi T)$ for different $\mathbf{k}$ as a function of $\delta$. This quantity serves as a rough marker for metallic ($\Delta\Sigma > 0$) or insulating ($\Delta\Sigma < 0$) behavior and confirms the gap opening at the point PG, corresponding in the noninteracting system to the intersection of the curve $\varepsilon(\mathbf{k}) = \mu$ with the Brillouin zone boundary. As discussed in the main text, the ARC momentum inside of the antiferromagnetic zone boundary is made more metallic by spin fluctuations down to the smallest dopings. The small slope of $\mu(\delta)$ in panel (c) of Fig. S.3 at small dopings indicates an enhanced compressibility $\partial\delta/\partial\mu$. The latter is often observed near the critical point of the phase separation instability of strongly correlated Hubbard models [64–72].

Fig. S.3 (b) shows the leading eigenvalues as a function of doping. As discussed above, the largest eigenvalue corresponds to the charge channel at $\mathbf{q} = 0$ and $\omega = 2\pi T$. In our physical setting it can be interpreted as a measure of 'Mottness' [cf. Eq. (S.9)], as it leads to a divergence of the charge vertex at the zero temperature Mott transition [23]. This eigenvalue increases when approaching half-filling, even more steeply as the pseudogap opens. The next largest eigenvalue is in the spin channel for $\omega = 0$ where the corresponding momentum depends on doping, leading to a relay race of incommensurate momenta with decreasing $\delta$. The commensurate momentum $\mathbf{Q} = (\pi,\pi)$ [$(8,8)$ in Fig. S.3 b)] becomes the leading instability at roughly $\delta = 0.03$. Panel (d) shows the screened interaction $W(\mathbf{q},\omega = 0)$ on the high-symmetry path ($W = W^{\rm sp}$). Corresponding to the crossover from incommensurate to commensurate momenta $W$ develops from a two-peak structure to a single large peak (corresponding to 8 and 4 peaks in the Brillouin zone, respectively). The correlation length, estimated from the width of the peak, is indicated for dopings $\delta = 0.05, 0.04, 0.03, 0.02,$ and $0.01$.

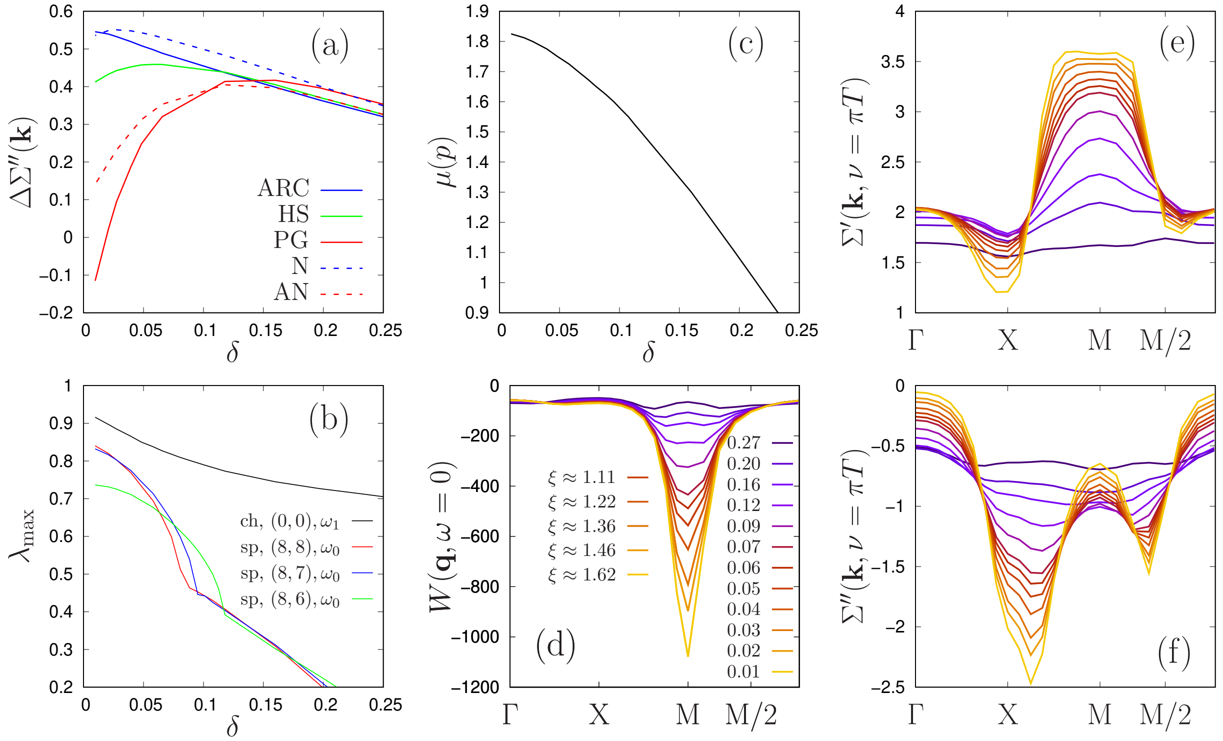


Supplementary Figure S.3: Various observables (see text) corresponding to a doping scan ($x$-axis or color code in the panels) as calculated in the parquet dual fermion approach for the Hubbard model with $U/t = 8, t = 1, t' = -0.2t, t'' = 0.1t$. The temperature is set to $T/t = 0.15$, the lattice size is $N = 16 \times 16$.

Finally, panels (e) and (f) show the real, respectively imaginary part of self-energy for various dopings. At large doping the self-energy is almost local but acquires a strong momentum dependence closer to half-filling. The spatial resolution is sufficient to differentiate the antinode $\mathrm{X} = (\pi, 0)$ from the position PG where the pseudogap opens first, which lies two units away from X. Similarly, a second peak is located not at the node $\mathrm{M}/2 = (\pi/2, \pi/2)$ but instead lies closer to the corner of the Brillouin zone, $(\pi/2 + \epsilon, \pi/2 + \epsilon)$.

### B. Imaginary part of the spin-fermion vertex in the ladder approximation

In the main text the imaginary part of the spin-fermion vertex $\Gamma$ plays an important role, because it facilitates the strong-coupling mechanism that allows spin fluctuations to open the pseudogap beginning near the antinodes. In the weak-coupling picture the gap opens first at the hot spots [73] and hence $\Gamma''$ is large only for strong coupling. To show this we calculate $\Gamma$ within the ladder dual fermion approximation according to Eq. (S.8), which is cheap and easy to converge. As before, the temperature is set to $T/t = 0.15$. The left panel of Fig. S.4 shows the ratio,

$$\frac{\Gamma''(\nu = \pi T, \mathbf{q} = \mathbf{Q}, \omega = 0)}{\Gamma'(\nu = \pi T, \mathbf{q} = \mathbf{Q}, \omega = 0)}. \tag{S.26}$$

Large negative values near half-filling indicate that the strong-coupling mechanism may play a role in the formation of the pseudogap. Notice that the ratio $\Gamma''/\Gamma'$ corresponds to an odd function of $\nu$ (see main text), its value at fixed $\nu_0 = \pi T$ therefore decreases with $T$ (unless it develops a pole at zero which we do not observe in our parquet and ladder calculations).

### C. Diagrammatic analysis of the local spin-fermion vertex

We derive an approximation for the imaginary part of the static spin-fermion vertex $\Gamma_{\mathrm{loc}}(\nu, \omega = 0)$ of the AIM and test it in practice. According to Ref. [74] the vertex correction due to single-boson exchange in the vertical

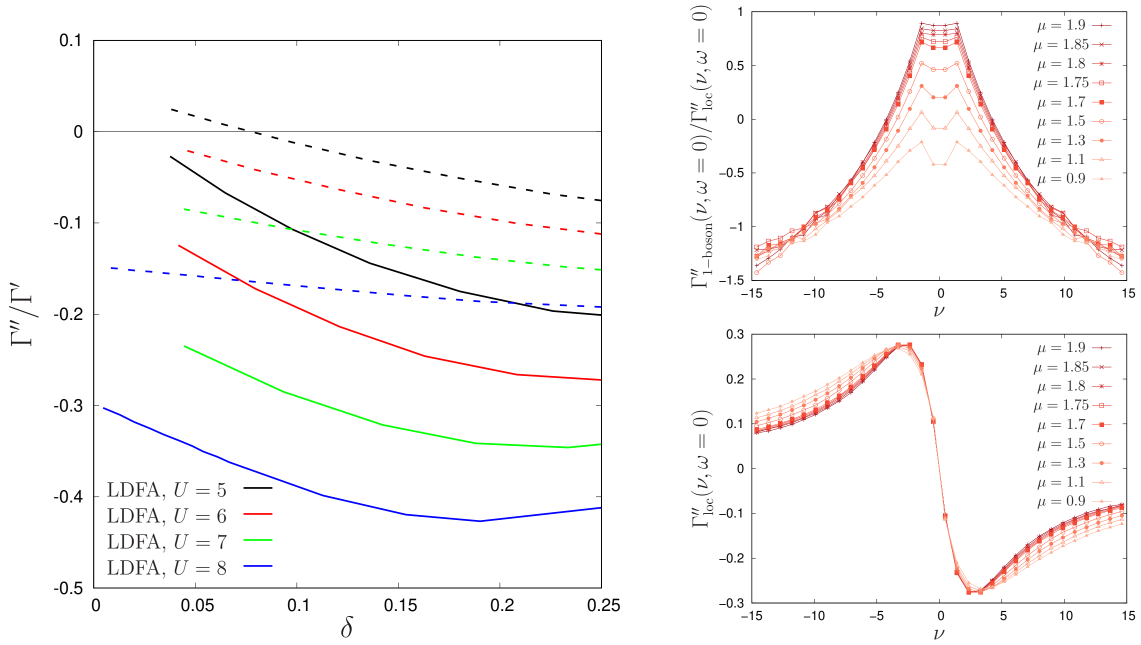


Supplementary Figure S.4: Left: Ratio of imaginary over real part of the spin-fermion vertex calculated in the ladder approximation (full lines) for various $U$ and $\delta$ ($t=1$, $t'=-0.2t$, $t''=0.1t$). Frequencies are set to $\nu=\pi T$, $\omega=0$, the bosonic momentum to $\mathbf{Q}=(\pi,\pi)$. In the ladder approximation the vertex does not depend on the fermionic momentum $\mathbf{k}$. Dashed lines correspond to the momentum-independent spin-fermion vertex $\Gamma_{\mathrm{loc}}$ of the AIM. A large $\Gamma''$ is a hallmark of the strong-coupling regime, nonlocal correlations further enhance this quantity. Top right: Approximation Eq. (S.27) for the imaginary part of the local spin-fermion vertex $\Gamma_{\mathrm{loc}}$ of the AIM. Bottom right: Imaginary part of the exact local spin-fermion vertex calcualted numerically by continuous-time quantum Monte Carlo.

particle-hole channel is given as,

$$\Gamma_{1-\mathrm{boson}}(\nu,\omega=0) = 1+\sum_{\nu'}[\nabla^{\overline{ph}}(\nu,\nu')+U]g(\nu')g(\nu'), \tag{S.27}$$

$$\nabla^{\overline{ph}}(\nu,\nu') = -\frac{1}{2}\Gamma^{\mathrm{ch}}_{\mathrm{loc}}(\nu,\nu'-\nu)w^{\mathrm{ch}}(\nu'-\nu)\Gamma^{\mathrm{ch}}_{\mathrm{loc}}(\nu,\nu'-\nu)+\frac{1}{2}\Gamma_{\mathrm{loc}}(\nu,\nu'-\nu)w(\nu'-\nu)\Gamma_{\mathrm{loc}}(\nu,\nu'-\nu). \tag{S.28}$$

We are interested in a rough estimate of the imaginary part. To this end, we introduce a few further approximations: the contribution due to charge fluctuations is neglected, $\Gamma^{\mathrm{ch}}_{\mathrm{loc}}(\nu,\nu'-\nu)w^{\mathrm{ch}}(\nu'-\nu)\Gamma^{\mathrm{ch}}_{\mathrm{loc}}(\nu,\nu'-\nu)\approx U$, the spin-fermion vertex is set to 1 on the right-hand-side of Eq. (S.27), and only contributions of static spin fluctuations are taken into account, $w(\omega)\approx -U-\frac{U^2}{2}\chi^{\mathrm{sp}}(\omega=0)\delta_\omega$. With these simplifications Eq. (S.27) reads,

$$\Gamma_{1-\mathrm{boson}}(\nu,\omega=0) \approx 1-\frac{TU^2}{4}\chi^{\mathrm{sp}}(\omega=0)g(\nu)g(\nu), \tag{S.29}$$

where the factor $T$ was implicit in the Matsubara summation. Taking the imaginary part we arrive at the approximation discussed in the main text.

Here we test this approximation in the DMFT calculations which serve as the basis for the dual parquet solver. For implementation reasons we evaluate Eq. (S.27) instead of (S.29). The ratio $\Gamma''_{1-\mathrm{boson}}(\nu,\omega=0)/\Gamma''_{\mathrm{loc}}(\nu,\omega=0)$ is drawn on the top right panel of Fig. S.4. Actually, it is close to unity only for small frequencies and values of the chemical potential where the pseudogap opens ($\mu\approx 1.8$). The drastic change of the approximation quality is remarkable in view of the weak $\mu$-dependence of the numerically exact $\Gamma''_{\mathrm{loc}}$ shown in the bottom right panel [75]. In any case, we employ Eq. (S.29) in the main text only for the lowest Matsubara frequencies to underline that $\Gamma$ develops a large imaginary part at strong coupling.

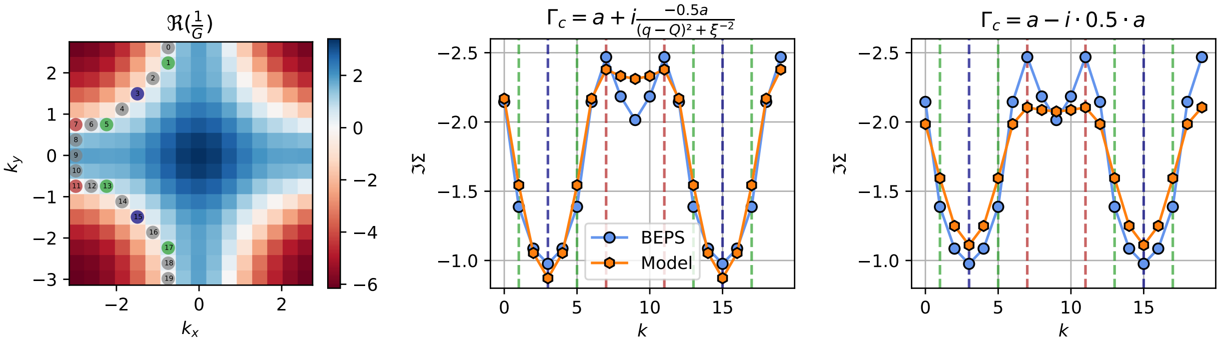


Supplementary Figure S.5: Comparison of the model self-energy (S.30) to the numerical pseudogap self-energy was obtained by parquet dual fermion at hole-doping $\delta = 0.01$.

## D. Comparison of model self-energy to numerical results

We compare the model self-energy, introduced in Eq. (4) of our main text, to the self-energy shown in Fig. 3(c) of the main text, corresponding to the pseudogap regime at doping $\delta = 0.01$. To avoid analytical continuation, we consider only the first Matsubara frequency,

$$\Sigma_{\rm sp}(\mathbf{k}, \pi T) \propto \frac{T}{N}\sum_{\mathbf{q}}\Gamma_c \frac{G^0(\mathbf{k}+\mathbf{q}, \pi T)}{(\mathbf{Q}-\mathbf{q})^2+\xi^{-2}}. \tag{S.30}$$

The scattering vector $\mathbf{Q} = (\pi, \pi)$ and the correlation length $\xi \approx 1.6$ are taken from our numerical calculation. For the prefactor, which includes the vertex correction $\Gamma(\nu, \omega = 0)$, we assume a complex number $\Gamma_c = a(1 - 0.5\imath)$. We then perform a least-squares fit of the prefactor $a$ to our numerical result (for the fit we considered only the relevant momenta $\mathbf{k}$ explicitly marked in the left panel of Fig. S.5). Using this $\Gamma_c$ we obtain the fit shown in the right panel of Fig. S.5.

The overall agreement is reasonable, however, it should be remarked that according to our numerical calculation the vertex $\Gamma(\mathbf{k}, \mathbf{q}, \nu, \omega = 0)$ displays a nontrivial momentum structure. In particular, its imaginary part is peaked near $\mathbf{q} \approx \mathbf{Q}$, compare bottom panels of Fig. 4 of the main text. We assume that the width of the peak corresponds roughly to the correlation length $\xi$, which yields our model for the prefactor, $\Gamma_c(\mathbf{q}) = a(1 - \frac{0.5\imath}{(\mathbf{Q}-\mathbf{q})^2+\xi^{-2}})$. Taking into account this $\mathbf{q}$-dependence, we obtain the fit shown in the center panel of Fig. S.5.

## E. Analytical continuation

Finally, we present in Fig. S.6 the analytical continuation $\imath\nu_n \to \nu + \imath\eta$ of the Green's function and self-energy to real frequencies $\nu$ for two exemplary momenta: in the nodal (ARC) and antinodal (PG) direction (the exact momenta are printed in the figure's legend). To this end, we use a Padé approximant based on the lowest 7 Matsubara frequencies of our parquet dual fermion calculation, and employ a broadening parameter $\eta = 0.01$. Because of the typical inaccuracy of the Padé fit for higher frequencies, we concentrate here on the behavior around the Fermi level from $-t$ to $+t$, which is anyhow the most important region as far as the pseudogap region is concerned. In order to avoid the additional, and in principle uncontrolled, uncertainty of the analytic continuation procedure, and considering that we are mostly interested in the momentum dependence of the self-energy at the Fermi surface, in the main manuscript we present (with the exception of Fig. 6) data at small but finite $\imath\nu_0 = \imath\pi T$, i.e., at the lowest Matsubara frequency.


[1] Friedrich Krien, Angelo Valli, Patrick Chalupa, Massimo Capone, Alexander I. Lichtenstein, and Alessandro Toschi, "Boson-exchange parquet solver for dual fermions," Phys. Rev. B **102**, 195131 (2020).

[2] A. N. Rubtsov, M. I. Katsnelson, and A. I. Lichtenstein, "Dual fermion approach to nonlocal correlations in the hubbard model," Phys. Rev. B **77**, 033101 (2008).

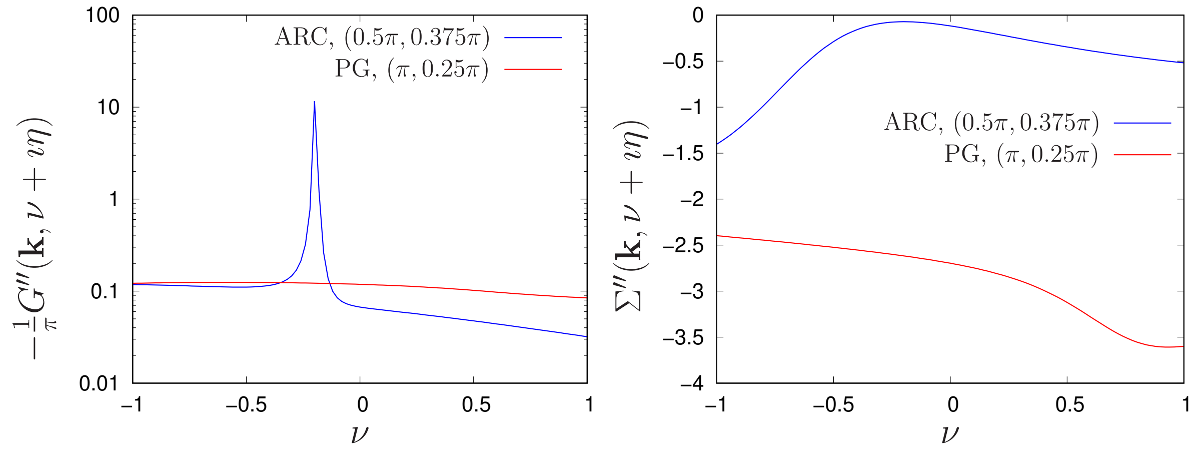


Supplementary Figure S.6: Spectral density (left) and imaginary part of the self-energy (right) for real frequencies $\nu$ (in units of $t$), computed for the ARC and the PG momentum in the pseudogap regime. The parameters are the same as in Fig. 6 of the main manuscript, i.e., doping $\delta = 0.01$, $t = 1, t' = -0.2t, t'' = 0.1t, U = 8t, T = 0.15t$. The huge imaginary part of the self-energy for the PG momentum (right) completely dampens the quasparticle peak for momenta in the PG region. A well-defined peak right below the Fermi level is still present for the ARC (see left panel).

[3] A. Toschi, A. A. Katanin, and K. Held, "Dynamical vertex approximation: A step beyond dynamical mean-field theory," Phys. Rev. B **75**, 045118 (2007).
[4] G. Rohringer, A. Toschi, H. Hafermann, K. Held, V. I. Anisimov, and A. A. Katanin, "One-particle irreducible functional approach: A route to diagrammatic extensions of the dynamical mean-field theory," Phys. Rev. B **88**, 115112 (2013).
[5] C. Taranto, S. Andergassen, J. Bauer, K. Held, A. Katanin, W. Metzner, G. Rohringer, and A. Toschi, "From infinite to two dimensions through the functional renormalization group," Phys. Rev. Lett. **112**, 196402 (2014).
[6] Thomas Ayral and Olivier Parcollet, "Mott physics and spin fluctuations: A unified framework," Phys. Rev. B **92**, 115109 (2015).
[7] G. Rohringer, H. Hafermann, A. Toschi, A. A. Katanin, A. E. Antipov, M. I. Katsnelson, A. I. Lichtenstein, A. N. Rubtsov, and K. Held, "Diagrammatic routes to nonlocal correlations beyond dynamical mean field theory," Rev. Mod. Phys. **90**, 025003 (2018).
[8] Antoine Georges, Gabriel Kotliar, Werner Krauth, and Marcelo J. Rozenberg, "Dynamical mean-field theory of strongly correlated fermion systems and the limit of infinite dimensions," Rev. Mod. Phys. **68**, 13–125 (1996).
[9] B Bauer, L D Carr, H G Evertz, A Feiguin, J Freire, S Fuchs, L Gamper, J Gukelberger, E Gull, S Guertler, A Hehn, R Igarashi, S V Isakov, D Koop, P N Ma, P Mates, H Matsuo, O Parcollet, G Pawowski, J D Picon, L Pollet, E Santos, V W Scarola, U Schollwöck, C Silva, B Surer, S Todo, S Trebst, M Troyer, M L Wall, P Werner, and S Wessel, "The alps project release 2.0: open source software for strongly correlated systems," Journal of Statistical Mechanics: Theory and Experiment **2011**, P05001 (2011).
[10] Hartmut Hafermann, Kelly R. Patton, and Philipp Werner, "Improved estimators for the self-energy and vertex function in hybridization-expansion continuous-time quantum monte carlo simulations," Phys. Rev. B **85**, 205106 (2012).
[11] P. Gunacker, M. Wallerberger, E. Gull, A. Hausoel, G. Sangiovanni, and K. Held, "Continuous-time quantum monte carlo using worm sampling," Phys. Rev. B **92**, 155102 (2015).
[12] Markus Wallerberger, Andreas Hausoel, Patrik Gunacker, Alexander Kowalski, Nicolaus Parragh, Florian Goth, Karsten Held, and Giorgio Sangiovanni, "w2dynamics: Local one- and two-particle quantities from dynamical mean field theory," Computer Physics Communications **235**, 388 – 399 (2019).
[13] H. Hafermann, G. Li, A. N. Rubtsov, M. I. Katsnelson, A. I. Lichtenstein, and H. Monien, "Efficient perturbation theory for quantum lattice models," Phys. Rev. Lett. **102**, 206401 (2009).
[14] T. Ribic, P. Gunacker, S. Iskakov, M. Wallerberger, G. Rohringer, A. N. Rubtsov, E. Gull, and K. Held, "Role of three-particle vertex within dual fermion calculations," Phys. Rev. B **96**, 235127 (2017).
[15] T. Schäfer, G. Rohringer, O. Gunnarsson, S. Ciuchi, G. Sangiovanni, and A. Toschi, "Divergent precursors of the mott-hubbard transition at the two-particle level," Phys. Rev. Lett. **110**, 246405 (2013).
[16] Erik G. C. P. van Loon, Friedrich Krien, and Andrey A. Katanin, "Bethe-salpeter equation at the critical end point of the mott transition," Phys. Rev. Lett. **125**, 136402 (2020).
[17] Friedrich Krien, "Efficient evaluation of the polarization function in dynamical mean-field theory," Phys. Rev. B **99**, 235106 (2019).
[18] Erik G. C. P. van Loon, Mikhail I. Katsnelson, and Hartmut Hafermann, "Second-order dual fermion approach to the mott transition in the two-dimensional hubbard model," Phys. Rev. B **98**, 155117 (2018).

[19] Erik G C P van Loon, "Second-order dual fermion for multi-orbital systems," Journal of Physics: Condensed Matter **33**, 135601 (2021).
[20] Grigory V. Astretsov, Georg Rohringer, and Alexey N. Rubtsov, "Dual parquet scheme for the two-dimensional hubbard model: Modeling low-energy physics of high-$T_c$ cuprates with high momentum resolution," Phys. Rev. B **101**, 075109 (2020).
[21] Sergei Iskakov, Andrey E. Antipov, and Emanuel Gull, "Diagrammatic monte carlo for dual fermions," Phys. Rev. B **94**, 035102 (2016).
[22] Jan Gukelberger, Evgeny Kozik, and Hartmut Hafermann, "Diagrammatic monte carlo approach for diagrammatic extensions of dynamical mean-field theory: Convergence analysis of the dual fermion technique," Phys. Rev. B **96**, 035152 (2017).
[23] Friedrich Krien, Erik G. C. P. van Loon, Mikhail I. Katsnelson, Alexander I. Lichtenstein, and Massimo Capone, "Two-particle fermi liquid parameters at the mott transition: Vertex divergences, landau parameters, and incoherent response in dynamical mean-field theory," Phys. Rev. B **99**, 245128 (2019).
[24] C. Husemann, K.-U. Giering, and M. Salmhofer, "Frequency-dependent vertex functions of the $(t, t^{'})$ hubbard model at weak coupling," Phys. Rev. B **85**, 075121 (2012).
[25] Demetrio Vilardi, Ciro Taranto, and Walter Metzner, "Nonseparable frequency dependence of the two-particle vertex in interacting fermion systems," Phys. Rev. B **96**, 235110 (2017).
[26] M. Reitner, P. Chalupa, L. Del Re, D. Springer, S. Ciuchi, G. Sangiovanni, and A. Toschi, "Attractive effect of a strong electronic repulsion: The physics of vertex divergences," Phys. Rev. Lett. **125**, 196403 (2020).
[27] Václav Janiš, Anna Kauch, and Vladislav Pokorný, "Thermodynamically consistent description of criticality in models of correlated electrons," Phys. Rev. B **95**, 045108 (2017).
[28] Ar. Abanov, Andrey V. Chubukov, and J. Schmalian, "Quantum-critical theory of the spin-fermion model and its application to cuprates: Normal state analysis," Advances in Physics **52**, 119–218 (2003), https://doi.org/10.1080/0001873021000057123.
[29] P. A. Igoshev, A. A. Katanin, and V. Yu. Irkhin, "Magnetic fluctuations and itinerant ferromagnetism in two-dimensional systems with van hove singularities," Journal of Experimental and Theoretical Physics **105**, 1043–1056 (2007).
[30] A. A. Katanin, "Nonanalytic momentum dependence of spin susceptibility for heisenberg magnets in the paramagnetic phase and its effect on critical exponents," Phys. Rev. B **103**, 054415 (2021).
[31] N. E. Bickers and D. J. Scalapino, "Critical behavior of electronic parquet solutions," Phys. Rev. B **46**, 8050–8056 (1992).
[32] Alan J. Bray, "Self-consistent screening calculation of the critical exponent $\eta$," Phys. Rev. Lett. **32**, 1413–1416 (1974).
[33] Lorenzo Del Re, Massimo Capone, and Alessandro Toschi, "Dynamical vertex approximation for the attractive hubbard model," Phys. Rev. B **99**, 045137 (2019).
[34] Thomas Schäfer, Nils Wentzell, Fedor Šimkovic, Yuan-Yao He, Cornelia Hille, Marcel Klett, Christian J. Eckhardt, Behnam Arzhang, Viktor Harkov, François-Marie Le Régent, Alfred Kirsch, Yan Wang, Aaram J. Kim, Evgeny Kozik, Evgeny A. Stepanov, Anna Kauch, Sabine Andergassen, Philipp Hansmann, Daniel Rohe, Yuri M. Vilk, James P. F. LeBlanc, Shiwei Zhang, A.-M. S. Tremblay, Michel Ferrero, Olivier Parcollet, and Antoine Georges, "Tracking the footprints of spin fluctuations: A multimethod, multimessenger study of the two-dimensional hubbard model," Phys. Rev. X **11**, 011058 (2021).
[35] Friedrich Krien, Alexander I. Lichtenstein, and Georg Rohringer, "Fluctuation diagnostic of the nodal/antinodal dichotomy in the hubbard model at weak coupling: A parquet dual fermion approach," Phys. Rev. B **102**, 235133 (2020).
[36] Friedrich Krien, Angelo Valli, and Massimo Capone, "Single-boson exchange decomposition of the vertex function," Phys. Rev. B **100**, 155149 (2019).
[37] Christian J. Eckhardt, Carsten Honerkamp, Karsten Held, and Anna Kauch, "Truncated unity parquet solver," Phys. Rev. B **101**, 155104 (2020).
[38] Chu-Xin Chen and N.E. Bickers, "Numerical solution of parquet equations for the anderson impurity model," Solid State Communications **82**, 311 – 315 (1992).
[39] S. X. Yang, H. Fotso, J. Liu, T. A. Maier, K. Tomko, E. F. D'Azevedo, R. T. Scalettar, T. Pruschke, and M. Jarrell, "Parquet approximation for the $4 \times 4$ hubbard cluster," Phys. Rev. E **80**, 046706 (2009).
[40] Ka-Ming Tam, H. Fotso, S.-X. Yang, Tae-Woo Lee, J. Moreno, J. Ramanujam, and M. Jarrell, "Solving the parquet equations for the hubbard model beyond weak coupling," Phys. Rev. E **87**, 013311 (2013).
[41] A. Valli, T. Schäfer, P. Thunström, G. Rohringer, S. Andergassen, G. Sangiovanni, K. Held, and A. Toschi, "Dynamical vertex approximation in its parquet implementation: Application to hubbard nanorings," Phys. Rev. B **91**, 115115 (2015).
[42] Gang Li, Nils Wentzell, Petra Pudleiner, Patrik Thunström, and Karsten Held, "Efficient implementation of the parquet equations: Role of the reducible vertex function and its kernel approximation," Phys. Rev. B **93**, 165103 (2016).
[43] Herbert F Fotso, Ka-Ming Tam, and Juana Moreno, "Beyond quantum cluster theories: Multiscale approaches for strongly correlated systems," (2020), arXiv:2011.05522.
[44] Gang Li, Anna Kauch, Petra Pudleiner, and Karsten Held, "The victory project v1.0: An efficient parquet equations solver," Computer Physics Communications **241**, 146–154 (2019).
[45] C. Husemann and M. Salmhofer, "Efficient parametrization of the vertex function, $\Omega$ scheme, and the $t, t^{'}$ hubbard model at van hove filling," Phys. Rev. B **79**, 195125 (2009).
[46] Wan-Sheng Wang, Yuan-Yuan Xiang, Qiang-Hua Wang, Fa Wang, Fan Yang, and Dung-Hai Lee, "Functional renormalization group and variational monte carlo studies of the electronic instabilities in graphene near $\frac{1}{4}$ doping," Phys. Rev. B **85**, 035414 (2012).

[47] J. Lichtenstein, D. Snchez de la Pea, D. Rohe, E. Di Napoli, C. Honerkamp, and S.A. Maier, "High-performance functional renormalization group calculations for interacting fermions," Computer Physics Communications **213**, 100 – 110 (2017).

[48] C. J. Eckhardt, G. A. H. Schober, J. Ehrlich, and C. Honerkamp, "Truncated-unity parquet equations: Application to the repulsive hubbard model," Phys. Rev. B **98**, 075143 (2018).

[49] Friedrich Krien, Anna Kauch, and Karsten Held, "Tiling with triangles: parquet and $gw\gamma$ methods unified," Phys. Rev. Research **3**, 013149 (2021).

[50] O. Gunnarsson, T. Schäfer, J. P. F. LeBlanc, E. Gull, J. Merino, G. Sangiovanni, G. Rohringer, and A. Toschi, "Fluctuation diagnostics of the electron self-energy: Origin of the pseudogap physics," Phys. Rev. Lett. **114**, 236402 (2015).

[51] O. Gunnarsson, T. Schäfer, J. P. F. LeBlanc, J. Merino, G. Sangiovanni, G. Rohringer, and A. Toschi, "Parquet decomposition calculations of the electronic self-energy," Phys. Rev. B **93**, 245102 (2016).

[52] Georg Rohringer, "Spectra of correlated many-electron systems: From a one- to a two-particle description," Journal of Electron Spectroscopy and Related Phenomena **241**, 146804 (2020), sources, Interaction with Matter, Detection and Analysis of Low Energy Electrons (SIMDALEE2).

[53] Thomas Schfer and Alessandro Toschi, "How to read between the lines of electronic spectra: the diagnostics of fluctuations in strongly correlated electron systems," Journal of Physics: Condensed Matter **33**, 214001 (2021).

[54] Lorenzo Del Re and Georg Rohringer, "Fluctuations diagnostic of the spin susceptibility: Neel ordering revisited in dmft," (2021), arXiv:2104.11737 [cond-mat.str-el].

[55] Behnam Arzhang, A. E. Antipov, and J. P. F. LeBlanc, "Fluctuation diagnostics of the finite-temperature quasi-antiferromagnetic regime of the two-dimensional hubbard model," Phys. Rev. B **101**, 014430 (2020).

[56] T. Ribic, P. Gunacker, and K. Held, "Impact of self-consistency in dual fermion calculations," Phys. Rev. B **98**, 125106 (2018).

[57] Rok Žitko, "Convergence acceleration and stabilization of dynamical mean-field theory calculations," Phys. Rev. B **80**, 125125 (2009).

[58] Hugo U. R. Strand, Andro Sabashvili, Mats Granath, Bo Hellsing, and Stellan Östlund, "Dynamical mean field theory phase-space extension and critical properties of the finite temperature mott transition," Phys. Rev. B **83**, 205136 (2011).

[59] Josef Kaufmann, Christian Eckhardt, Matthias Pickem, Motoharu Kitatani, Anna Kauch, and Karsten Held, "Self-consistent ladder dynamical vertex approximation," (2021).

[60] Amartya S. Banerjee, Phanish Suryanarayana, and John E. Pask, "Periodic pulay method for robust and efficient convergence acceleration of self-consistent field iterations," Chemical Physics Letters **647**, 31–35 (2016).

[61] M. Grilli and C. Castellani, "Electron-phonon interactions in the presence of strong correlations," Phys. Rev. B **50**, 16880–16898 (1994).

[62] F. Becca, M. Tarquini, M. Grilli, and C. Di Castro, "Charge-density waves and superconductivity as an alternative to phase separation in the infinite-u hubbard-holstein model," Phys. Rev. B **54**, 12443–12457 (1996).

[63] P. Chalupa, T. Schäfer, M. Reitner, D. Springer, S. Andergassen, and A. Toschi, "Fingerprints of the local moment formation and its kondo screening in the generalized susceptibilities of many-electron problems," Phys. Rev. Lett. **126**, 056403 (2021).

[64] Nobuo Furukawa and Masatoshi Imada, "Charge gap, charge susceptibility and spin correlationin the hubbard model on a square lattice," Journal of the Physical Society of Japan **60**, 3604–3607 (1991), https://doi.org/10.1143/JPSJ.60.3604.

[65] Nobuo Furukawa and Masatoshi Imada, "Charge mass singularity in two-dimensional hubbard model," Journal of the Physical Society of Japan **62**, 2557–2560 (1993), https://doi.org/10.1143/JPSJ.62.2557.

[66] G. Kotliar, Sahana Murthy, and M. J. Rozenberg, "Compressibility divergence and the finite temperature mott transition," Phys. Rev. Lett. **89**, 046401 (2002).

[67] Martin Eckstein, Marcus Kollar, Michael Potthoff, and Dieter Vollhardt, "Phase separation in the particle-hole asymmetric hubbard model," Phys. Rev. B **75**, 125103 (2007).

[68] E. Khatami, K. Mikelsons, D. Galanakis, A. Macridin, J. Moreno, R. T. Scalettar, and M. Jarrell, "Quantum criticality due to incipient phase separation in the two-dimensional hubbard model," Phys. Rev. B **81**, 201101 (2010).

[69] Takahiro Misawa and Masatoshi Imada, "Origin of high-$T_c$ superconductivity in doped hubbard models and their extensions: Roles of uniform charge fluctuations," Phys. Rev. B **90**, 115137 (2014).

[70] Junya Otsuki, Hartmut Hafermann, and Alexander I. Lichtenstein, "Superconductivity, antiferromagnetism, and phase separation in the two-dimensional hubbard model: A dual-fermion approach," Phys. Rev. B **90**, 235132 (2014).

[71] Luca de' Medici, "Hund's induced fermi-liquid instabilities and enhanced quasiparticle interactions," Phys. Rev. Lett. **118**, 167003 (2017).

[72] R. Nourafkan, M. Ct, and A. M. S. Tremblay, "Charge-fluctuations in lightly hole-doped cuprates: effect of vertex corrections," (2018), arXiv:1807.03855.

[73] Wei Wu, Mathias S. Scheurer, Shubhayu Chatterjee, Subir Sachdev, Antoine Georges, and Michel Ferrero, "Pseudogap and fermi-surface topology in the two-dimensional hubbard model," Phys. Rev. X **8**, 021048 (2018).

[74] Friedrich Krien and Angelo Valli, "Parquetlike equations for the hedin three-leg vertex," Phys. Rev. B **100**, 245147 (2019).

[75] Notice that Eq. (S.27) is nowhere suitable as an approximation for the real part, $\Gamma'_{\mathrm{loc}}$ (not shown).
